# Supplementary material for: LLM Support for Mathematical Problem Posing: What Changes When Revision Formulations Are Supplied or Withheld?
Source: arXiv:2607.09628 source file (2026-11-22)
Supplement: Supplementary file 1 [file appendix.tex]

| Interview code | Coded utterances | Unique participants | Participants |
|---|---:|---:|---|
| `socratic-deeper-thinking` | 16 | **5/20 (25%)** | MC04, MC05, MC06, MC10, MC16 |
| `direct-efficiency` | 20 | **8/20 (40%)** | MC01, MC02, MC03, MC04, MC05, MC08, MC09, MC10 |
| `Socratic-confusing-unexpected-response` | 12 | **7/20 (35%)** | MC02, MC03, MC04, MC05, MC08, MC17, MC20 |
| `desired-switch-point` | 6 | **4/20 (20%)** | MC03, MC05, MC13, MC18 |
